# Supplementary material for: Policy-Gradient Training of Fair and Unbiased Ranking Functions
Source: arXiv:1911.08054 source file (2021-05-09)
Supplement: Supplementary file 1 [file appendix.tex]

\clearpage
\appendix
\section{Discussion}
\subsection{Alternate Definition of Disparity} \label{subsec:alt_def_disparity_appendix}
An alternate path towards a closely related disparity measure using implicit feedback is the following. We replace the query-specific exposure and merit with an amortized notion of exposure and merit~\cite{BiegaGW18:EquityAttention} over the query distribution
\begin{equation*}
	\frac{\E_{q}[\exposure_q(G_i|\pi)]}{\E_{q}\left[\merit_q({G_i})\right]}=\frac{\E_{q}[\exposure_q(G_j|\pi)]}{\E_{q}\left[\merit_q({G_j})\right]}.
\end{equation*}
This constraint expresses that for all the queries, the amortized exposure of each group should be proportional to its amortized merit. We will show that the disparity 
% \begin{equation}
% 	\label{eqn:disp2}
% 	D'_{ij}(\pi)=\frac{\E_{q}[\exposure_q(G_i|\pi)]}{\E_{q}[\merit_q({G_i})]}-\frac{\E_{q}[\exposure_q(G_j|\pi)]}{\E_{q}[\merit_q({G_j})]}
% \end{equation}
is equivalent to disparity measure $D_{ij}(\pi)$ defined in the previous section under two assumptions. First, assume that the total exposure of both groups is a constant $\exposure_q(G_i)+\exposure_q(G_j)=C_E$. In practice, the top items receive most of the users' attention, so the total exposure for each query is relatively stable even if the size of the candidate set varies. Secondly, assume that the covariance of the exposure of group $G_j$ and the total number of relevant items in both groups, $\cov[\exposure(G_j|\pi),\merit_q(G_i)+\merit_q(G_j)]$, is zero. One sufficient condition for this assumption to be approximately satisfied is when the numbers of relevant items do not vary much between queries. Under these two assumptions, the disparity measures $D_{ij}(\pi)$ and $D'_{ij}(\pi)$ are equivalent up to a constant coefficient
\begin{equation*}
	D_{ij}(\pi)=\E_q[{\merit_q(G_i)}]\E_q[\merit_q(G_j)]D'_{ij}(\pi).
\end{equation*}
This can be shown by transforming the disparity measure $D'_{ij}(\pi)$ as follows,
\begin{align*}
	&\frac{\E_{q}\left[\exposure_q(G_i|\pi)\right]}{\E_{q}[\merit_q(G_i)]}-\frac{\E_{q}[\exposure_q(G_j|\pi)]}{\E_{q}[\merit_q(G_j)]}\\
	=& \frac{\E_{q}[\exposure_q(G_i|\pi)]\E_q[\merit_q(G_j)]-\E_{q}[\exposure_q(G_j|\pi)]\E_q[\merit_q(G_i)]}{\E_{q}[\merit_q(G_i)]\E_{q}[\merit_q(G_j)]}\\
	=& \frac{D_{ij}(\pi)+\cov[\exposure_q(G_j|\pi), \merit_q(G_i)]-\cov[\exposure_q(G_i|\pi), \merit_q(G_j)]}{\E_{q}[\merit_q(G_i)]\E_{q}[\merit_q(G_j)]}.
\end{align*}
The difference between the covariance terms is zero,
\begin{align*}
	&\cov[\exposure_q(G_j|\pi), \merit_q(G_i)]-\cov[\exposure_q(G_i|\pi), \merit_q(G_j)]\\
    =&\cov[\exposure_q(G_j|\pi), \merit_q(G_i)]-\cov[C_E-\exposure_q(G_j|\pi), \merit_q(G_j)]\\
	=&\cov[\exposure(G_j|\pi),\merit_q(G_i)+\merit_q(G_j)]=0.
\end{align*}
Therefore, we have $D_{ij}(\pi)=\E_q[{\merit_q(G_i)}]\E_q[\merit_q(G_j)]D'_{ij}(\pi)$.

Note that we can also get a consistent estimator of $D'_{ij}(\pi)$ by using the IPS estimator of merit and replacing the expectations of exposure and merit with the average over the dataset
\begin{equation*}
	\widehat{D}'_{ij}(\pi|\queryset)=\frac{\sum_{q\in\queryset}\exposure_q(G_i|\pi)}{\sum_{q\in\queryset}\widehat{\merit}_q({G_i})}-\frac{\sum_{q\in\queryset}\exposure_q(G_j|\pi)}{\sum_{q\in\queryset}\widehat{\merit}_q({G_j})}.
\end{equation*}
As $N$ increases, $\widehat{D}'_{ij}(\pi|\queryset)$ will converge to $D'_{ij}(\pi)$. However, the estimator is not unbiased, which means $\E[\widehat{D}'_{ij}(\pi|\queryset)]\neq D'_{ij}(\pi)$. This bias might increase the error of the estimator. We therefore prefer the disparity $D_{ij}(\pi)$ with its unbiased estimator $\widehat{D}_{ij}(\pi)$, as defined in \Cref{eqn:group_disparity_estimator,eqn:group_disparity_emp}.
%Moreover, we need to compute $\sum_q\widehat{\relevance}_q({G_i})$ for each group $G_i$ in advance, which is infeasible or impossible for large datasets or in online setting where the training data arrives as a stream. On the other hand, our disparity measure as defined in \Cref{eqn:disparity_measure} can be applied in online settings and its IPS estimator in \Cref{eqn:group_disparity_estimator} is shown to be unbiased.
\subsection{Disparity Estimator With Noise} \label{subsec:noise_appendix}
We show that the disparity estimator is not order preserving with noise.
\begin{align*}
	&\E_{c_q}\left[\widehat{\merit}_q(G_i)\exposure_q(G_j|\pi)\right]\\
	=&\E_{o_q}\E_{c_q|o_q}\Bigg[\sum_{d\in G_i^q}(c_q(d)/p)\exposure_q(G_j|\pi)\Bigg]\\
	=&{\sum_{d\in G_i^q}\left[\epsilon_+\merit_q(d)+\epsilon_-(1-\merit_q(d))\right]}{\exposure_q(G_j|\pi)}\\
	=&(\epsilon_+-\epsilon_-){\merit_q(G_i)}{\exposure_q(G_j|\pi)}+\epsilon_-|G_i^q|{\exposure_q(G_j|\pi)},
\end{align*}
where $p$ stands for $p(o_q(d)=1|{r}_q)$. The expectation of the disparity estimator with click noise is
\begin{align*}
	&\E_{c_q}\left[\widehat{D}_{ij}(\pi|q)\right]\\
	=&(\epsilon_+-\epsilon_-)\left({\merit_q(G_j)}{\exposure_q(G_i|\pi)}-{\merit_q(G_i)}{\exposure_q(G_j|\pi)}\right)\\
	&+\epsilon_-\left(|G_j^q|{\exposure_q(G_i|\pi)}-|G_i^q|{\exposure_q(G_j|\pi)}\right)\\
	=&(\epsilon_+-\epsilon_-)D_{ij}(\pi|q)+\epsilon_-\left(|G_j^q|{\exposure_q(G_i|\pi)}-|G_i^q|{\exposure_q(G_j|\pi)}\right).
\end{align*}
The additional term is dependent on the policy $\pi$. Therefore, the disparity estimator is not order-preserving,

\begin{align*}
	\E_q\!\!\left[\widehat{D}_{ij}(\pi_1|\queryset)-\widehat{D}_{ij}(\pi_2|\queryset)\right]& \!=(\epsilon_+\!-\!\epsilon_-)\E_{q}\!\!\left[D_{ij}(\pi_1|\queryset)-D_{ij}(\pi_2|\queryset)\right]\\
	&\!\!\!\!\!\!\!\!\!\!\!\!\!\!\!+\epsilon_-\E_{q}\!\!\left[|G_j^q|\delta\exposure_q(G_i)-|G_i^q|\delta\exposure_q(G_j)\right],
\end{align*}
where $\delta\exposure(G_i^q)$ stands for ${\exposure_q(G_i|\pi_1)}-{\exposure_q(G_i|\pi_2)}$. This implies that when $\epsilon_-=0$, our IPS estimator for group disparity is consistent for finding an optimal ranking policy regardless of the value of $\epsilon_+$. However, when $\epsilon_->0$, the disparity estimator is not order-preserving, which means that there can exist two policies $\pi_1$ and $\pi_2$ such that $\E\big[D_{ij}(\pi_1|\queryset)\big]>\E\big[D_{ij}(\pi_2|\queryset)\big]$ but $\widehat{D}_{ij}(\pi_1)<\widehat{D}_{ij}(\pi_2)$.

Given the expectation of $\widehat{D}_{ij}(\pi|q)$ under click noise, it is straightforward to show the corrected disparity estimator in \Cref{eqn:noise-free} is unbiased up to a constant factor $\epsilon_+-\epsilon_-$.
\begin{align*}
	&\E_{c_q}\left[\widehat{D}_{ij}(\pi|q,\epsilon_-)\right]\\
	=&\E_{c_q}\left[\widehat{D}_{ij}(\pi|q)\right]-\epsilon_-\left(|G_j^q|{\exposure_q(G_i|\pi)}-|G_i^q|{\exposure_q(G_j|\pi)}\right).\\
	=&(\epsilon_+-\epsilon_-)D_{ij}(\pi|q)
\end{align*}

\section{Experiment Setting}
\label{sec:setting}

\subsection{Baseline Implementation}
\label{subsec:implementation}
In the utility evaluation in \Cref{subsec:utility-evaluation}, we compare FULTR with the following LTR baselines:
\begin{itemize}
  \item LambdaRank~\cite{LambdaRank:BurgesRL06}: Since no official implementation is available, we implement LambdaRank with PyTorch in our code. The searched hyperparameters are the L2 regularization coefficient and the learning rate.
  \item Propensity SVM-Rank~\cite{PropSVMRank:JoachimsSS17}: We use the official implementation released by the authors \footnote{\url{http://www.cs.cornell.edu/people/tj/svm_light/svm_proprank.html}}. The searched hyperparameter is the regularization coefficient $C$.
  \item PG-Rank~\cite{PolicyFairness:abs-1902-04056}: We implement it with PyTorch in our code. The searched hyperparameter is the L2 regularization coefficient.
\end{itemize}

In the fairness evaluation in \Cref{subsec:fairness-evaluation}, we compare FULTR with the following fair ranking baselines:
\begin{itemize}
	\item Group-blind: It is implemented by masking the group attribute of the input to \model~ without any fairness constraint.
	\item Fair-PG-Rank~\cite{PolicyFairness:abs-1902-04056}: We implement it with PyTorch in our code. The searched hyperparameter is the L2 regularization coefficient.
	\item Equity of Attention~\cite{BiegaGW18:EquityAttention}: Since no official implementation is available, we implement the algorithm based on integer linear programming using the Gurobi software \footnote{\url{http://www.gurobi.com}}, following the instructions in the paper. Since the post-processing method requires relevances for all items, we train a regression model $r(x_q(d))$ on all the query-item pairs in the training set using an unbiased IPS objective for relevance estimation proposed in \cite{underreview2019}. The IPS objective for relevance estimation is:
	\begin{equation*}
		\begin{split}
			\mathcal{L} = \sum_{q}\sum_{d\in d^q}\Big([r(x_q(d))]^2-\frac{2c_q(d)}{p}r(x_q(d))+\frac{c_q(d)}{p}\Big).
		\end{split}
	\end{equation*}
\end{itemize}
